# Supplementary material for: Real-Time Diffusion Policies for Games: Enhancing Consistency Policies with Q-Ensembles
Source: arXiv:2503.16978 source file (2025-03-21)
Supplement: Supplementary file 1 [file appendix.tex]

\section{Appendix}
\label{sec:appendix}

\section{Hyperparameters}
